# Supplementary material for: Iterative Pre-Conditioning for Expediting the Gradient-Descent Method: The Distributed Linear Least-Squares Problem
Source: arXiv:2008.02856 source file (2021-08-06)
Supplement: Supplementary file 1 [file appendix.tex]

%%%%%%%%%%%%%%%%%%%%%%%%%%%%%%%%%%%%%%%%%%%%%%%%%%%%%%%%%%%%%%%%%%%%%%%%%%%%%%%%
\section{APPENDIX}

%\printcomment{ ++++ can we add the theorem and lemma statements here for easy verification +++++}

%%%%%%%%%%%%%%%%%%%%%%%%%%%%%%%%%%%%%%%%%%%%%%%
\noindent \fbox{\begin{minipage}{\textwidth}
\begin{theorem} \label{thm:thm1}
Consider Algorithm 1 with $\beta > 0$. Then, for arbitrary $x(0)$ and $K(-1)$:
\begin{itemize}
    \item There exists $\delta > 0$ for which there is a positive value $\rho_{\beta} < 1$ such that
\begin{align}
    \norm{z(t+1)^{\perp}} \leq \left(\rho_{\beta}+\sigma_0 (\rho^*_K)^{t+1}\right) \norm{z(t)^{\perp}}, \, \forall t, \label{eqn:zperp_6}
\end{align}
where $\rho_{\beta} \geq \ro$.
    \item $\underset{t \rightarrow \infty}{lim} \, z(t)^{\perp} = 0$.
    \item $x(t)$ converges to a solution of~\eqref{eqn:opt_1} as $t \rightarrow \infty$.
\end{itemize}
\end{theorem}
\end{minipage}}

\subsection{Proof of Theorem~\ref{thm:thm1}}
\label{prf:thm1}

We begin with the following claim which shows that, each column of the pre-conditioner matrix $K(t)$ asymptotically converges to the corresponding column of $K^*_{\beta}$. In other words, the matrix $K(t)$ asymptotically converges to $K^*_{\beta}$.\\

\noindent \fbox{\begin{minipage}{\textwidth}
\begin{claim} \label{thm:clm1}
Consider the iterative process~\eqref{eqn:kcol_update}, and let $\beta > 0$. Then, there exists $\alpha > 0$ for which there is a positive value $\rho_K < 1$ such that for each $j=1,\ldots,d$,
\begin{align*}
    \norm{k_j(t)-k_j^*} \leq \rho_K \norm{k_j(t-1)-k_j^*}, \, t=0,1,2,\ldots,
\end{align*}
where $\rho_K \geq \rho^*_K$.
\end{claim}
\end{minipage}}
~\\

\begin{proof}
Observing that $A^T A = \sum_{i=1}^m (A^i)^T A^i$ and $A^T b = \sum_{i=1}^m (A^i)^T b^i$, from~\eqref{eqn:Rij} we have
\[ \sum_{i=1}^m R^i_j(t) = \left[\left(\A+\beta I\right)k_j(t) - e_j\right]. \]
Then, dynamics~\eqref{eqn:kcol_update} can be rewritten as
\begin{align} \label{eqn:kcol_2}
    k_j(t) & = k_j(t-1) - \alpha \left[\left(\A+\beta I\right)k_j(t-1) - e_j\right].
\end{align}
Define $\Tilde{k}_j(t) := k_j(t) - k_j^*$. From the definition of $K^*_{\beta}$ we have,
\begin{align*}
    \left(\A+\beta I\right)K^*_{\beta} = I \implies \left(\A+\beta I\right) k_j^* = e_j, \, j=1,...,d.
\end{align*}
From~\eqref{eqn:kcol_2} then we have,
\begin{align}
    \Tilde{k}_j(t) = \left[I- \alpha \left(\A+\beta I\right)\right] \Tilde{k}_j(t-1).
\end{align}
Since $(\A+\beta I)$ is positive definite for $\beta >0$, $\exists \alpha$ for which there is a positive $\rho_K < 1$ such that $\norm{\Tilde{k}_j(t)} \leq \rho_K \norm{\Tilde{k}_j(t-1)}$, $t=0,1,2,...$, where the smallest value of $\rho_K$ is $\dfrac{\kappa(\A+\beta I)-1}{\kappa(\A+\beta I)+1}$ (ref. Corollary 11.3.3 and Chapter 11.3.3 of~\cite{fessler2008image}). As $\kappa(\A+\beta I)=\dfrac{\lambda+\beta}{\gamma+\beta}$, the claim follows.
\end{proof}

We state some facts from linear algebra that is required for the next part of the proof.
From the fundamental theorem of linear algebra, $\R^n = \mathcal{N}(\A) \oplus \mathcal{N}(\A)^{\perp}$. Then, for every there $v \in \R^n$ there is a unique decomposition
\begin{align}
    v = v^{\mathcal{N}} + v^{\perp}, \label{eqn:decomp}
\end{align}
where $v^{\mathcal{N}} \in \mathcal{N}(\A)$ is the component of $v$ in the kernel of $\A$ and $v^{\perp} \in \mathcal{N}(\A)^{\perp}$ is the component of $v$ in the orthogonal complement of kernel of $\A$. \\

Using~\eqref{eqn:g_i}, and observing that $A^T A = \sum_{i=1}^m (A^i)^T A^i$ and $A^T b = \sum_{i=1}^m (A^i)^T b^i$, dynamics~\eqref{eqn:x_update} can be rewritten as
\begin{align}
    x(t+1) & = x(t) - \delta K(t) A^T\left(Ax(t)-b\right). \label{eqn:x_central}
\end{align}
The objective cost in~\eqref{eqn:opt_1} can be rewritten as $\dfrac{1}{2}\norm{A \, x -b}^2$, gradient of which is given by $\A x - A^T b$. Thus, $x^*$ satisfies $\A \, x^* = A^T b$.
From~\eqref{eqn:err},~\eqref{eqn:x_central}, and $\A \, x^* = A^T b$, we get
\begin{align}
    z(t+1) & = \left(I- \delta K(t)\A\right) z(t). \label{eqn:z_mltp}
\end{align}
Consider the singular value decomposition $\A = V S V^T$, where 
%$V \in \R^{n \times n}$ and 
$V \in \R^{d \times d}$
is unitary and %$S = \begin{bmatrix} S_1 & \mathbf{O} \end{bmatrix} \in \R^{d \times d}$ with $S_1 = diag\{\sigma_1,...,\sigma_d\}$
$S = diag\{\lambda_1,...,\lambda_d\} \in \R^{d \times d}$
is the diagonal matrix consisting of the singular values $\lambda_i \geq 0$ of the positive semi-definite matrix $\A$. Let the rank of $\A$ be denoted by $r$. Then, $\lambda_1 \geq ... \geq \lambda_r > \lambda_{r+1} = ... = \lambda_d = 0$. 
Let $\{v_i\}_{i=1}^d$ be the right singular vectors of $\A$, i.e., $V = \begin{bmatrix} v_1 ... v_d \end{bmatrix}$. 
Define a  matrix $V_r := \begin{bmatrix} v_1 ... v_r \end{bmatrix}$.
It is known that, the orthogonal projection matrix onto $\mathcal{N}(\A)^{\perp}$ is $V_r V_r^T =: Q$ (ref. Section 2.5.2 of\cite{golub2012matrix}). Define a diagonal matrix
\[ S^{\perp} := diag\{ \underbrace{1,...,1}_r \, \underbrace{0,...,0}_{d-r} \}. \]
Then, $Q$ can be also expressed as $Q = V S^{\perp} V^T $.
From the definition of $Q$,
\begin{align}
    z(t+1)^{\perp} & = Q \, z(t+1) \nonumber \\
    & \overset{\eqref{eqn:z_mltp}}{=} Q \, z(t) - \delta Q K(t)\A \, z(t) \nonumber \\
    & = z(t)^{\perp} - \delta Q K(t)\A \, \left(z(t)^{\mathcal{N}} + z(t)^{\perp} \right) \nonumber \\
    & = z(t)^{\perp} - \delta Q K(t)\A \, z(t)^{\perp}, \nonumber
\end{align}
where the last equality follows from $z(t)^{\mathcal{N}} \in \mathcal{N}(\A)$.
Let $\Tilde{K}(t)$ comprise of the columns $\Tilde{k}_j(t) := k_j(t) - k_j^*$, $j=1,...,d$. Then,
\begin{align}
    z(t+1)^{\perp} & = z(t)^{\perp} - \delta Q K^*_{\beta}\A \, z(t)^{\perp} - \delta Q \Tilde{K}(t)\A \, z(t)^{\perp} \nonumber \\
    \implies \norm{z(t+1)^{\perp}} & \leq \norm{z(t)^{\perp} - \delta \underbrace{V S^{\perp} V^T}_Q K^*_{\beta}\A \, z(t)^{\perp}} + \norm{\delta Q \Tilde{K}(t)\A \, z(t)^{\perp}}. \label{eqn:zperp_1}
\end{align}
From Lemma~\ref{thm:lem1}, it follows that
\begin{align}
    & \norm{\Tilde{k}^j(t)}^2 \leq (\rho^*_K)^{2t+2} \norm{\Tilde{k}^j(-1)}^2, \, j=1,...,dd  \nonumber \\
    \implies & \norm{\Tilde{K}(t)}_F^2 = \sum_{j=1}^d \norm{\Tilde{k}^j(t)}^2 \leq \sum_{j=1}^d (\rho^*_K)^{2t+2} \norm{\Tilde{k}^j(-1)}^2 = (\rho^*_K)^{2t+2} \norm{\Tilde{K}(-1)}_F^2 \nonumber \\
    \implies & \norm{\Tilde{K}(t)} \leq \norm{\Tilde{K}(t)}_F \leq (\rho^*_K)^{t+1} \norm{\Tilde{K}(-1)}_F. \label{eqn:K_frob}
\end{align}
It is known that, a projection matrix has unity 2-norm (follows form (5.9.8) of~\cite{meyer2000matrix}). Then,
\begin{align}
    \norm{\delta Q \Tilde{K}(t)\A \, z(t)^{\perp}} & \leq \delta \norm{Q} \norm{\Tilde{K}(t)} \norm{\A} \norm{z(t)^{\perp}} \nonumber \\
    & = \delta \norm{\Tilde{K}(t)} \underbrace{\norm{\A}}_\lambda \norm{z(t)^{\perp}} \nonumber \\
    & \overset{\eqref{eqn:K_frob}}{\leq} \underbrace{\delta \lambda \norm{\Tilde{K}(-1)}_F}_{\sigma_0} \, (\rho^*_K)^{t+1} \norm{z(t)^{\perp}}, \label{eqn:z_perp_rhs}
\end{align}
where the equality follows from $Q$ being a projection matrix.

The vectors in $V_r$ form an orthonormal basis of $\mathcal{N}(A)^{\perp}$. Since $z(t)^{\perp} \in \mathcal{N}(A)^{\perp}$ by definition, we can express $z(t)^{\perp}$ as a linear combination of the basis vectors in $V_r$:
\begin{align}
    z(t)^{\perp} = \sum_{i=1}^r \underbrace{<z(t)^{\perp}, v_i>}_{=:z_i} \, v_i, \label{eqn:z_lc}
\end{align}
where $<.\,,\,.>$ denotes the Euclidean inner product. 
\begin{comment} 
Using the singular value decomposition of $A$ and $U$ being orthonormal, we have
\begin{align*}
    \A = (USV^T)^T(USV^T) = VS^TSV,
\end{align*}
which is known as the eigen decomposition of $\A$. So, $S^TS = diag\{\lambda_1,...,\lambda_d\} =: \Sigma$, where $\lambda_k = \sigma_k^2 \geq 0$ are the eigenvalues of positive semi-definite matrix $\A$. 
\end{comment} 
Since $K^*_{\beta} := \left(\A+\beta I\right)^{-1}$ and the identity matrix can be written as $I=V V^T$, from the singular value decomposition of $\A$ we have 
\begin{align}
    & K^*_{\beta} = V \, diag\{\dfrac{1}{\lambda_{k}+\beta}\}_{k=1}^d \, V^T \nonumber \\
    \implies & K^*_{\beta}\A = V \, diag\{\dfrac{1}{\lambda_{k}+\beta}\}_{k=1}^d \, V^T V \, diag\{\lambda_{k}\}_{k=1}^n \, V^T \nonumber \\
    \implies & K^*_{\beta}\A = V \, \underbrace{diag\{\dfrac{\lambda_{k}}{\lambda_{k}+\beta}\}_{k=1}^d}_{=:\Lambda} \, V^T.  \label{eqn:eig_dec_KA}
\end{align}
Then,
\begin{align}
    z(t)^{\perp} - \delta V S^{\perp} V^T K^*_{\beta}\A \, z(t)^{\perp} & \overset{\eqref{eqn:eig_dec_KA}}{=} z(t)^{\perp} - \delta  V S^{\perp} \underbrace{V^T V}_I \Lambda V^T z(t)^{\perp} \nonumber \\
    & = z(t)^{\perp} - \delta  V S^{\perp} \Lambda V^T z(t)^{\perp} \nonumber \\
    & = z(t)^{\perp} - \delta  V \Lambda^{\perp} \, V^T z(t)^{\perp}, \label{eqn:zperp_2}
\end{align}
where $\Lambda^{\perp} := diag\{ \underbrace{\mu_1,...,\mu_r}_r \, \underbrace{0,...,0}_{d-r} \}$, and $\mu_k := \dfrac{\lambda_{k}}{\lambda_{k}+\beta}$.
Using the expansion $V \Lambda^{\perp} \, V^T = \sum_{i=1}^r \mu_i v_i v_i^T$ and plugging~\eqref{eqn:z_lc} into~\eqref{eqn:zperp_2},
\begin{align}
    z(t)^{\perp} - \delta V S^{\perp} V^T K^*_{\beta}\A \, z(t)^{\perp} & = \sum_{i=1}^r z_i v_i - \delta \sum_{i=1}^r \mu_i v_i v_i^T z(t)^{\perp} \nonumber \\
    & = \sum_{i=1}^r z_i v_i - \delta \sum_{i=1}^r \mu_i v_i <z(t)^{\perp}, v_i> \nonumber \\
    & = \sum_{i=1}^r z_i v_i - \delta \sum_{i=1}^r \mu_i v_i z_i \nonumber \\
    & = \sum_{i=1}^r \left(1-\delta \mu_i \right) z_i v_i \nonumber
\end{align}
Using orthonormality of $V$,
\begin{align}
     \norm{z(t)^{\perp} - \delta V S^{\perp} V^T K^*_{\beta}\A \, z(t)^{\perp}}^2 & = \sum_{i=1}^r \left(1-\delta \mu_i \right)^2 z_i^2 \norm{v_i}^2 = \sum_{i=1}^r \left(1-\delta \mu_i \right)^2 z_i^2 \leq \rho_{\beta}^2 \sum_{i=1}^r z_i^2, \label{eqn:zperp_3} 
\end{align}
where $\rho_{\beta} := \underset{1\leq k \leq r}{max} \mnorm{1-\delta \mu_k}$.
Since $\sigma_1 \geq ... \geq \sigma_r > 0$ and $\lambda_k = \sigma_k^2$, we then have
\[ \lambda_1 \geq ... \geq \lambda_r > 0. \]
Since $\dfrac{d}{d\lambda_k}(\mu_k) = \dfrac{d}{d\lambda_k} \left(\dfrac{\lambda_{k}}{\lambda_{k}+\beta}\right) > 0$ and $\lambda_1 \geq ... \geq \lambda_r > 0$, we have
\[\mu_1 \geq ... \geq \mu_r > 0. \]
If $\delta \in \left(0,\dfrac{2}{\mu_1}\right)$, then $\mnorm{1-\delta \mu_k} < 1, \, k=1,...,r $. Furthermore, $\rho_{\beta} = max\{\mnorm{1-\delta \mu_1},\mnorm{1-\delta \mu_r}\} < 1$ and the smallest value of $\rho_{\beta}$ is given by $\ro := \dfrac{\mu_1-\mu_r}{\mu_1+\mu_r}$ (ref. Chapter 11.3.3 of~\cite{fessler2008image}).

From~\eqref{eqn:z_lc} and orthonormality of $V$,
\begin{align}
    \norm{z(t)^{\perp}}^2 = \norm{\sum_{1=1}^r z_i v_i}^2 = \sum_{1=1}^r z_i^2 \norm{v_i}^2 = \sum_{1=1}^r z_i^2. \label{eqn_zperp_4}
\end{align}
From~\eqref{eqn:zperp_3} and~\eqref{eqn_zperp_4},
\begin{align}
    & \norm{z(t)^{\perp} - \delta V S^{\perp} V^T K^*_{\beta}\A \, z(t)^{\perp}}^2 \leq \rho_{\beta}^2 \norm{z(t)^{\perp}}^2 \nonumber\\
    \implies & \norm{z(t)^{\perp} - \delta V S^{\perp} V^T K^*_{\beta}\A \, z(t)^{\perp}} \leq \rho_{\beta} \norm{z(t)^{\perp}}. \label{eqn:zperp_5} 
\end{align}
Combining~\eqref{eqn:zperp_1},~\eqref{eqn:z_perp_rhs} and~\eqref{eqn:zperp_5}, we get
\begin{align*}
    \norm{z(t+1)^{\perp}} \leq \rho_{\beta} \norm{z(t)^{\perp}} + \sigma_0 (\rho^*_K)^{t+1} \norm{z(t)^{\perp}} = \left(\rho_{\beta} + \sigma_0 (\rho^*_K)^{t+1} \right) \norm{z(t)^{\perp}},
\end{align*}
which is~\eqref{eqn:zperp_6}.
Plugging in $\mu_k = \dfrac{\lambda_{k}}{\lambda_{k}+\beta}$ in $\ro := \dfrac{\mu_1-\mu_r}{\mu_1+\mu_r}$, where $\lambda_1 = \lambda$ and $\gamma_r = \lambda_r$ are respectively the largest and smallest non-zero eigenvalues of $\A$,  the first statement of the theorem follows. \\

\underline{For the second statement,} denote the rate of convergence by $\alpha_t := \left(\rho_{\beta}+\sigma_0 (\rho^*_K)^{t+1} \right)$. Since $\rho_K^* < 1$, $\{\alpha_t > 0\}_{t \geq 0}$ is strictly decreasing sequence and $\lim_{t \rightarrow \infty}\alpha_t = \rho_{\beta} < 1$. \\

\noindent \fbox{\begin{minipage}{\textwidth}
\begin{claim} \label{thm:clm2}
Consider a sequence $\{x_t > 0\}_{t \geq 0}$ such that $x_t < x_{t-1} \, \forall t$ and $\lim_{t \rightarrow \infty} x_t < L$. Then, there exists $T' < \infty$ such that $x_t < L \, \forall t > T'$.
\end{claim}
\end{minipage}}
~\\

\begin{proof}
This can be shown by contradiction. Note that, the claim is equivalent to $x_t < L$ for some finite $t$, because $x_t < x_{t-1} \, \forall t$. Assume, $x_t \geq L \, \forall t < \infty$. Then the infimum of the sequence $\{x_t: t < \infty\}$ is L. Since the real sequence $\{x_t: t < \infty\}$ is lower bounded by zero and strictly decreasing, its infimum is the limit of the sequence (follows from the Monotone Convergence Theorem of Real Sequences). But $\lim_{t \rightarrow \infty} x_t < L$. This is a contradiction. 
\end{proof}

From the above claim, there exists a positive integer $\tau$ such that $\alpha_t < 1 \, \forall t > \tau$.
From~\eqref{eqn:zperp_6}, we get
\begin{align}
    & \norm{z(t+1)^{\perp}} \leq \left(\Pi_{k=\tau+1}^t \, \alpha_k\right) \norm{z(\tau + 1)^{\perp}}, \, \forall t > \tau. \label{eqn:zclm_1}
\end{align}
From~\eqref{eqn:zperp_6} and the fact that $\{\alpha_t > 0\}_{t \geq 0}$ is a strictly decreasing sequence, we have
\begin{align}
    & \norm{z(\tau+1)^{\perp}} \leq \alpha_{\tau} \norm{z(\tau)^{\perp}} \leq \alpha_{0} \norm{z(\tau)^{\perp}}, \nonumber \\
    \implies & \norm{z(\tau+1)^{\perp}} \leq \alpha_{0}^{\tau+1} \norm{z(0)^{\perp}}. \label{eqn:zclm_2}
\end{align}
Combining~\eqref{eqn:zclm_1} and~\eqref{eqn:zclm_2},
\begin{align*}
    \norm{z(t+1)^{\perp}} & \leq \left(\Pi_{k=\tau+1}^t \, \alpha_k\right) \alpha_{0}^{\tau+1} \norm{z(0)^{\perp}} \\
    & \leq \left(\Pi_{k=\tau+1}^t \, \alpha_{\tau +1}\right) \alpha_{0}^{\tau+1} \norm{z(0)^{\perp}} \\
    & = \alpha_{\tau+1}^t \left(\dfrac{\alpha_{0}}{\alpha_{\tau+1}}\right)^{\tau+1}, \, \forall t>\tau.
\end{align*}
Since $\alpha_{\tau+1} < 1$, we have $\underset{t \rightarrow \infty}{\lim} \, \alpha_{\tau+1}^t \left(\dfrac{\alpha_{0}}{\alpha_{\tau+1}}\right)^{\tau+1} = 0$ and the second statement of the theorem follows. \\

\underline{From $\underset{t \rightarrow \infty}{\lim} \, z(t)^{\perp} = 0$ we have},
\begin{align*}
    & \underset{t \rightarrow \infty}{\lim} \, z(t) = \underset{t \rightarrow \infty}{\lim} \, \left( z(t)^{\mathcal{N}} + z(t)^{\perp} \right) = \underset{t \rightarrow \infty}{\lim} \, z(t)^{\mathcal{N}} \\
    \iff &  \underset{t \rightarrow \infty}{\lim} \, x(t) - x^* = \underset{t \rightarrow \infty}{\lim} \, z(t)^{\mathcal{N}} \\
    \iff &  \underset{t \rightarrow \infty}{\lim} \, x(t) = x^* + \underset{t \rightarrow \infty}{\lim} \, z(t)^{\mathcal{N}}.
\end{align*}
But $\left(\underset{t \rightarrow \infty}{\lim} \, z(t)^{\mathcal{N}}\right) \in \mathcal{N}(\A)$ by definition. So, $x(t)$ converges to $\left(x^* + y \right)$ for some $y \in \mathcal{N}(\A)$ as $t \rightarrow \infty$. Now, $$\A\left(x^* + y \right) = \A x^* + \A y^* = A^T b + 0 = A^T b,$$
which means $\left(x^* + y \right)$ is a point of minima of~\eqref{eqn:opt_1}. Since we have shown that $x(t)$ converges to $\left(x^* + y \right)$, the third statement of the theorem follows.

%%%%%%%%%%%%%%%%%%%%%%%%%%%%%%%%%%%%%%%%%%%%%%%
\noindent \fbox{\begin{minipage}{\textwidth}
\begin{lemma} \label{thm:lem1}
Consider Algorithm~\ref{algo_1} and assume $\kappa(\A) > 1$. If $a=1$, then for $\beta > 0$ we have,
\begin{itemize}
    \item $r^{(a)} < 1$ and
\begin{align}
    \norm{z(t+1)^{\perp}} \leq c^{(a)} \left(r^{(a)} \, \rho^{(a)} \right)^{t+1} \, \norm{z(0)^{\perp}}, \, \forall t > \tau \label{eqn:z2_lem1}
\end{align}
    \item We have
    \begin{align}
    c^{(a)} \left(r^{(a)} \, \rho^{(a)} \right)^{t+1} < \left(\rho^{(a)}\right)^{t+1}, \, \forall t > t^{(a)}. \label{eqn:tsw_lem1}
\end{align}
\end{itemize}
If $a=2$, then~\eqref{eqn:z2_lem1} and~\eqref{eqn:tsw_lem1} hold for $\beta < \sqrt{3\lambda \gamma_r}$. If $a=3$, then~\eqref{eqn:z2_lem1} and~\eqref{eqn:tsw_lem1} hold for $\beta < \sqrt{\lambda \gamma_r}$.
\end{lemma}
\end{minipage}}

\subsection{Proof of Lemma~\ref{thm:lem1}}
\label{prf:lem1}

We make a claim that compares the convergence rate of two algorithms for solving~\eqref{eqn:opt_1}, both of them having time-varying rate of contraction, one of which is smaller than the other after a finite number of iterations. We refer these algorithms as Algorithm-I and Algorithm-II. Our result is a direct application of this claim, as will be shown shortly. \\

To present this claim, we define a few notations. 
\begin{itemize}
\setlength\itemsep{0.5em}
    \item Let the estimate of optimum point $x^*$ computed by Algorithm-I and Algorithm-II be denoted by $x_1(t)$ and $x_2(t)$, respectively, after $t$ iterations. 
    Define the estimation errors $z_1(t) := x_1(t)-x^*$ and $z_2(t) := x_2(t)-x^*$.
    \item The least upper-bound of $\norm{z_i(t)^{\perp}}, \, i=1,2,$ are as follows:
\begin{align}
    \norm{z_1(t+1)^{\perp}} & \leq \alpha_t \norm{z_1(t)^{\perp}} \, \text{and} \,
    \norm{z_2(t+1)^{\perp}} \leq \eta_t \norm{z_2(t)^{\perp}}, \, \forall t. \label{eqn:z1} 
\end{align}
    \item Define $r_t := \dfrac{\alpha_t}{\eta_t}$ and $\Bar{r} := \underset{t>\tau}{max} \, r_t$.
    \item Define
    \begin{align}
        c := \left(\dfrac{\alpha_{0}}{\Bar{r}}\right)^{\tau+1} \left(\dfrac{1}{\Pi_{k=0}^{\tau} \, \eta_k}\right), \, 
        t_{sw} := \floor{\dfrac{log \left(c \right)}{log \left(\dfrac{1}{\Bar{r}} \right)}}.
    \end{align}
\end{itemize}

\noindent \fbox{\begin{minipage}{\textwidth}
\begin{claim} \label{thm:clm3}
Suppose $\{\alpha_t > 0\}_{t \geq 0}$ is a strictly decreasing sequence such that $\alpha_t < \eta_t < 1 \, \forall t>\tau$. 
If both the algorithms are identically initialized with $x(0) \in \R^n$, then 
\begin{itemize}
    \item $\Bar{r} < 1$ and
\begin{align}
    \norm{z_1(t+1)^{\perp}} \leq c \left(\Bar{r}\right)^{t+1} \, \left(\Pi_{k=0}^{t} \, \eta_k\right) \, \norm{z(0)^{\perp}}, \, \forall t > \tau \label{eqn:z2}
\end{align}
    \item We have
    \begin{align}
    c \left(\Bar{r}\right)^{t+1} \, \left(\Pi_{k=0}^{t} \, \eta_k\right) < \left(\Pi_{k=0}^{t} \, \eta_k\right), \, \forall t > t_{sw}. \label{eqn:tsw}
\end{align}
\end{itemize}
\end{claim}
\end{minipage}}
~\\

\begin{proof}
From~\eqref{eqn:z1}, we get
\begin{align}
    & \norm{z_1(t+1)^{\perp}} \leq \left(\Pi_{k=\tau+1}^t \, \alpha_k\right) \norm{z_1(\tau + 1)^{\perp}}, \, \forall t > \tau. \label{eqn:z3}
\end{align}
From~\eqref{eqn:z1} and the fact that $\{\alpha_t > 0\}_{t \geq 0}$ is a strictly decreasing sequence, we have
\begin{align}
    & \norm{z_1(\tau+1)^{\perp}} \leq \alpha_{\tau} \norm{z_1(\tau)^{\perp}} \leq \alpha_{0} \norm{z_1(\tau)^{\perp}}, \nonumber \\
    \implies & \norm{z_1(\tau+1)^{\perp}} \leq \alpha_{0}^{\tau+1} \norm{z(0)^{\perp}}. \label{eqn:z4}
\end{align}
Combining~\eqref{eqn:z3} and~\eqref{eqn:z4},
\begin{align*}
    \norm{z_1(t+1)^{\perp}} & \leq \left(\Pi_{k=\tau+1}^t \, \alpha_k\right) \alpha_{0}^{\tau+1} \norm{z(0)^{\perp}} \\
    & = \left(\Pi_{k=\tau+1}^t \, r_k \eta_k\right) \alpha_{0}^{\tau+1} \norm{z(0)^{\perp}} \\
    & = \left(\Pi_{k=\tau+1}^t \, r_k \eta_k\right) \left(\Pi_{k=0}^{\tau} \, \eta_k\right) \left(\dfrac{\alpha_{0}^{\tau+1}}{\Pi_{k=0}^{\tau} \, \eta_k}\right) \norm{z(0)^{\perp}} \\
    & \leq \left(\Pi_{k=\tau+1}^t \, \Bar{r} \eta_k\right) \left(\Pi_{k=0}^{\tau} \, \eta_k\right) \left(\dfrac{\alpha_{0}^{\tau+1}}{\Pi_{k=0}^{\tau} \, \eta_k}\right) \norm{z(0)^{\perp}} \\
    & = \left(\Bar{r}\right)^{t-\tau} \left(\Pi_{k=0}^{t} \, \eta_k\right) \left(\dfrac{\alpha_{0}^{\tau+1}}{\Pi_{k=0}^{\tau} \, \eta_k}\right) \norm{z(0)^{\perp}} \\
    & = \left(\Bar{r}\right)^{t+1} \left(\Pi_{k=0}^{t} \, \eta_k\right) \, \underbrace{\left(\dfrac{\alpha_{0}}{\Bar{r}}\right)^{\tau+1} \left(\dfrac{1}{\Pi_{k=0}^{\tau} \, \eta_k}\right)}_c \, \norm{z(0)^{\perp}}, \, \forall t>\tau.
\end{align*}
Since $\alpha_t < \eta_t < 1 \, \forall t>\tau$, we have $r_t = \dfrac{\alpha_t}{\eta_t} < 1 \, \forall t>\tau$. Thus, $\Bar{r} := \underset{t>\tau}{max} \, r_t < 1$. This proves the first part of the claim.

%Since both $\Bar{r}, \, \eta_t \in (0,1)  \, \forall t>\tau$, we have $\underset{t \rightarrow \infty}{\lim} \, \left(\Bar{r}\right)^{t+1} \, \left(\Pi_{k=0}^{t} \, \eta_k\right) = 0$, and the second part of the clam follows from~\eqref{eqn:z2}.

Since $\Bar{r}< 1$, there exists $t_{sw} < \infty$ such that~\eqref{eqn:tsw} holds. To find an explicit form of $t_{sw}$, we want
\begin{align*}
    & c \left(\Bar{r}\right)^{t+1} \, \left(\Pi_{k=0}^{t} \, \eta_k\right) < \left(\Pi_{k=0}^{t} \, \eta_k\right) \\
    \iff & c \, \left(\Bar{r}\right)^{t+1} < 1 \\
    \iff & \left(\dfrac{1}{\Bar{r}} \right)^{t+1} > c \\
    \iff & t > \dfrac{log \left(c \right)}{log \left(\dfrac{1}{\Bar{r}} \right)} - 1.
\end{align*}
Hence, the least such integer $t_{sw}$ is given by $\floor{\dfrac{log \left(c \right)}{log \left(\dfrac{1}{\Bar{r}} \right)}}$, and the second part of the claim follows.
\end{proof}

\underline{For $a=1$}, consider Algorithm-I and Algorithm-II in Claim~\ref{thm:clm3} respectively to be Algorithm~\ref{algo_1} and the DGD algorithm. From Theorem~\ref{thm:thm1}, $\alpha_t = \left(\ro+\sigma_0 (\rho^*_K)^{t+1} \right)$. Moreover, $\eta_t = \rho^{(1)} = \rho_{GD} < 1, \, \forall t$. Since $\rho_K^* < 1$, $\{\alpha_t > 0\}_{t \geq 0}$ is strictly decreasing sequence and $\lim_{t \rightarrow \infty}\alpha_t = \ro$. From~\eqref{eqn:conv_dgd} and~\eqref{eqn:rho_def}, $\ro < \eta_t$ if $\beta > 0$ and $\kappa(\A)>1$. 
From Claim~\ref{thm:clm2} it follows that,there exists a positive integer $\tau^{(1)}$ such that $\alpha_t < \eta_t < 1 \, \forall t > \tau^{(1)}$. So, the conditions of Claim~\ref{thm:clm3} hold.

Define, $r_{t} := \dfrac{\alpha_{t}}{\eta_t}$. Then $r_t < 1 \, \forall t>\tau^{(1)}$. Since $\{\alpha_t > 0\}_{t \geq 0}$ is strictly decreasing sequence and $\eta_t$ is a constant, $\{r_t<1\}_{t>\tau^{(1)}}$ is a strictly decreasing sequence. 
So, $\Bar{r} = r_{\tau^{(1)}+1}$.

We have $\tau^{(1)}$ as the least integer satisfying $\alpha_{\tau+1} < \eta$. To get an explicit form of $\tau^{(1)}$:
\begin{align*}
    & \ro+\sigma_0 (\rho^*_K)^{\tau^{(1)}+1} < \rho^{(1)} \\
    \iff & \left(\dfrac{1}{\rho_K^*} \right)^{\tau^{(1)}+1} > \dfrac{\sigma_0}{\rho^{(1)} - \ro} \\
    \iff & \tau^{(1)} > \dfrac{log \left(\dfrac{\sigma_0}{\rho^{(1)} - \ro} \right)}{log \left(\dfrac{1}{\rho_K^*} \right)}-1.
\end{align*}
Noting from~\eqref{eqn:r_a} that $r^{(1)} = r_{\tau^{(1)}+1}$, the statement for $a=1$ follows from Claim~\ref{thm:clm3}. \\

For $a=2$ and $a=3$, we only need to show that $\ro < \rho^{(2)}$ and $\ro < \rho^{(3)}$ respectively hold for $\beta < \sqrt{3\lambda \gamma_r}$ and $\beta < \sqrt{\lambda \gamma_r}$, which is easy to verify. The statements for $a=2$ and $a=3$ then follow from the same argument as above for $a=1$. \\

\underline{For $a=2$} we want,
\begin{align*}
    \ro < \rho^{(2)} & \overset{\eqref{eqn:rho_def},\eqref{eqn:rho_nag}}{\iff} \dfrac{(\lambda - \gamma_r)\beta }{(\lambda + \gamma_r)\beta + 2\lambda \gamma_r} < 1 - \dfrac{2}{\sqrt{3\kappa(\A)+1}} \\
    & \iff \dfrac{\kappa(\A)-1}{\kappa(\A)+1 + 2\dfrac{\lambda}{\beta}} < 1 - \dfrac{2}{\sqrt{3\kappa(\A)+1}}.
\end{align*}
Let, $y^2:= \kappa(\A)$ and $p :=  2\dfrac{\lambda}{\beta}+1$. Then,
\begin{align*}
    \ro < \rho^{(2)} & \iff \dfrac{y^2-1}{y^2+p} + \dfrac{2}{\sqrt{3y^2+1}} -1 < 0 \\
    & \iff 2(y^2+p) < \sqrt{3y^2+1} \, (p+1).
\end{align*}
Let, $p=qy+1$ for some $q>0$. Then,
\begin{align*}
    \ro < \rho^{(2)} & \iff 2(y^2+qy+1) < \sqrt{3y^2+1} \, (qy+2) \\
    & \iff (y^2-1) \left(y(3q^2-4)+4q \right) > 0
\end{align*}
Since $y^2 =\kappa(\A) > 1$, we have
\begin{align*}
    \ro < \rho^{(2)} & \iff y(3q^2-4)+4q > 0.
\end{align*}
From the definitions of $p$ and $q$, we have $ q = \dfrac{2\lambda}{\beta y}$. Then,
\begin{align*}
    \ro < \rho^{(2)} & \iff 4y\left(\dfrac{3\lambda^2}{\beta^2 y^2}-1\right)+4q > 0.
\end{align*}
Now we show that, $\beta < \sqrt{3\lambda \gamma_r}$ satisfies the above condition.
\begin{align*}
    0 < \beta < \sqrt{3\lambda \gamma_r} & \iff \beta^2 < 3\lambda \gamma_r \\
    & \iff 1 < \dfrac{3\lambda \gamma_r}{\beta^2} = \dfrac{3\lambda^2\gamma_r}{\beta^2\lambda} = \dfrac{3\lambda^2}{\beta^2\kappa(\A)} = \dfrac{3\lambda^2}{\beta^2 y^2} \\
    & \implies 4y\left(\dfrac{3\lambda^2}{\beta^2 y^2}-1\right)+4q > 0 \iff \ro < \rho^{(2)},
\end{align*}
which is the desired condition. \\

\underline{For $a=3$}, we want
\begin{align*}
    \ro < \rho^{(3)} & \overset{\eqref{eqn:rho_def},\eqref{eqn:rho_hbm}}{\iff} \dfrac{(\lambda - \gamma_r)\beta }{(\lambda + \gamma_r)\beta + 2\lambda \gamma_r} < \dfrac{\sqrt{\kappa(\A)}-1}{\sqrt{\kappa(\A)}+1} \\
    & \iff \dfrac{\kappa(\A)-1}{\kappa(\A)+1 + 2\dfrac{\lambda}{\beta}} < \dfrac{\sqrt{\kappa(\A)}-1}{\sqrt{\kappa(\A)}+1} \\
    & \iff \left(\sqrt{\kappa(\A)}+1\right)^2 < \kappa(\A)+1 + 2\dfrac{\lambda}{\beta} \\
    & \iff \sqrt{\kappa(\A)} < \dfrac{\lambda}{\beta} \\
    & \iff \beta < \sqrt{\lambda \gamma_r},
\end{align*}
which is the desired condition.

%%%%%%%%%%%%%%%%%%%%%%%%%%%%%%%%%%%%%%%%%%%%%%%
\begin{comment}
\subsection{Proof of Theorem~\ref{thm:thm2}}
\label{prf:thm2}

Under Assumption 1, $\A$ is positive definite and $\left(\A\right)^{-1}$ is defined. Assumption 1 also implies that $\mathcal{N}(A) = \{\theta\}$ and $z(t) = z(t)^{\perp}$. Note that, $\rho_K^* = \rho_{GD}$ and $\ro = 0$ when $\beta = 0$. As Theorem~\ref{thm:thm1} holds true for $K^*_{\beta} = K^*_0$ and $\beta = 0$, from~\eqref{eqn:zperp_6} we obtain~\eqref{eqn:zperp_7}.

From~\eqref{eqn:zperp_7},
\begin{align*}
    \dfrac{\norm{z(t+1)}}{\norm{z(t)}} \leq \sigma_0 (\rho_{GD})^{t+1}.
\end{align*}
This implies that if $\rho_{GD} < 1$ then
\begin{align*}
    \underset{t \rightarrow \infty}{\lim} \, \dfrac{\norm{z(t+1)}}{\norm{z(t)}} \leq \underset{t \rightarrow \infty}{\lim} \, \sigma_0 (\rho_{GD})^{t+1} = 0.
\end{align*}
% which proves the second statement.
\end{comment}

%%%%%%%%%%%%%%%%%%%%%%%%%%%%%%%%%%%%%%%%%%%%%%%
\noindent \fbox{\begin{minipage}{\textwidth}
\begin{proposition} \label{thm:pro1}
Consider Algorithm~\ref{algo_1} with $\beta = 0$. If,
\begin{align}
    \rho_K^* < \rho_{j}, \, j=1,...,d \label{eqn:assump_2a}
\end{align}
and
\begin{align}
    w < w_{bd}. \label{eqn:assump_2b}
\end{align}
Then under Assumption 1,
\begin{itemize}
    \item there exists $T' < \infty$ such that
\begin{align}
    \lim_{t \rightarrow \infty} \norm{z(t)} < \dfrac{w}{1 - R(T'+1)}, \label{eqn:sse}
\end{align}
    where $t=T'$ is any integer satisfying $R(t+1) < 1$,% \, \forall t>T'$
    \item with
    \begin{align}
        \lim_{t \rightarrow \infty} \dfrac{w}{1 - R(T'+1)} = \dfrac{w}{1 - w/w_{bd}}. \label{eqn:sse_lim}
    \end{align}
\end{itemize}
\end{proposition}
\end{minipage}}

\subsection{Proof of Proposition 1}
\label{prf:pro1}

Due to noise,~\eqref{eqn:kcol_update} which is equivalent to~\eqref{eqn:kcol_2} becomes
\begin{align*}
    k^0_j(t) & = k_j(t-1) - \alpha \left[\left(\A+\beta I\right)k_j(t-1) - e_j\right].
\end{align*}
Then from Claim~\ref{thm:clm1} we have,
\begin{align*}
    \norm{\Tilde{k}^0_j(t)} & \leq (\rho^*_K) \norm{k_j(t-1)-k_j^*} \nonumber \\
    & = (\rho^*_K) \norm{k^o_j(t-1) + w^k_j(t) - k_j^*}, \nonumber \\
    & \leq (\rho^*_K) \norm{ k^o_j(t-1)- k_j^*} +(\rho^*_K) \norm{w^k_j(t)}, \nonumber \\
    & \leq (\rho^*_K)\norm{\Tilde{k}^0_j(t-1)} + (\rho^*_K) w, \, \forall t.
\end{align*}
Thus,
\begin{align}
    & \norm{\Tilde{k}^0_j(t)} \leq (\rho^*_K)^{t+1} \norm{\Tilde{k}^0_j(-1)} + \left(\rho^*_K+...+(\rho^*_K)^{t+1} \right)w \nonumber \\
    \implies & \norm{\Tilde{k}_j(t)} \leq (\rho^*_K)^{t+1} \norm{\Tilde{k}^0_j(-1)} + \left(1+\rho^*_K+...+(\rho^*_K)^{t+1} \right)w. \label{eqn:kcol_3}
\end{align}

Due to noise,~\eqref{eqn:x_update} which is equivalent to~\eqref{eqn:z_mltp} becomes
\begin{align}
    z^o(t+1) & = \left(I- \delta K(t)\A\right) z(t)  \nonumber \\
    & = \left(I- \delta K^*\A\right) \left( z^o(t)+w^x(t) \right) - \delta \Tilde{K}_t \A\, \left( z^o(t)+w^x(t) \right). \label{eqn:x1}
\end{align}
Now,
\begin{align*}
    & \norm{\Tilde{K}(t)}^2 \leq \norm{\Tilde{K}(t)}^2_F = \sum_{j=1}^d \norm{\Tilde{k}_j(t)}^2 \overset{\eqref{eqn:kcol_3}}{=} \underbrace{\sum_{j=1}^d \left( (\rho^*_K)^{t+1} \norm{\Tilde{k}^0_j(-1)} + \left(1+\rho^*_K+...+(\rho^*_K)^{t+1} \right)w \right)^2}_{S(t)^2} \\
    \implies & \norm{\Tilde{K}(t)} \leq S(t).
\end{align*}
Using the above bound and~\eqref{eqn:x1},
\begin{align*}
    \norm{z^o(t+1)} & \leq \underbrace{\ro}_{0} \left(\norm{z^o(t)}+w \right) + \delta S_t \norm{\A} \left(\norm{z^o(t)}+w \right) \\
    & = \underbrace{\delta S_t \lambda}_{R(t)} \left(\norm{z^o(t)}+w \right).
\end{align*}
Thus,
\begin{align}
    & \norm{z^o(t+1)} \leq R(t)...R(0) \norm{z^o(0)} + \left(R(t) + R(t) R(t-1) + ... + R(t)...R(0) \right)w \nonumber \\
    \implies & \norm{z(t+1)} \leq R(t)...R(0) \norm{z^o(0)} + \left(1+ R(t) + R(t) R(t-1) + ... + R(t)...R(0) \right)w \label{eqn:x2}
\end{align}

Define \[ p_j(t) := \left( (\rho^*_K)^{t+1} \norm{\Tilde{k}^0_j(-1)} + \left(1+\rho^*_K+...+(\rho^*_K)^{t+1} \right)w \right), \]
so that $S_t^2 = \sum_{j=1}^d p_j^2(t)$.
Then
\begin{align*}
    p_j(t) - p_j(t-1) & = \left((\rho^*_K)^{t+1} - (\rho^*_K)^{t}\right) \norm{\Tilde{k}^0_j(-1)} + (\rho^*_K)^{t+1} w \\
    & =  (\rho^*_K)^{t} \left((\rho^*_K) \left(w+\norm{\Tilde{k}^0_j(-1)}\right) - \norm{\Tilde{k}^0_j(-1)}\right) \\
    & \overset{\eqref{eqn:assump_2a}}{<} 0.
\end{align*}
Since $p_j(t) < p_j(t-1) \, \forall t, \, j = 1,...,d$, we have $S(t) < S(t-1) \, \forall t$ and hence $R(t) < R(t-1) \, \forall t$. 
Now
\begin{align}
    & \lim_{t \rightarrow \infty} S(t)^2 = \sum_{j=1}^d \left(\dfrac{1}{1-\rho_K^*}w \right)^2 = d \, \left(\dfrac{w}{1-\rho_K^*} \right)^2 \nonumber\\
    \implies & \lim_{t \rightarrow \infty} R(t) =  \dfrac{\delta \lambda \sqrt{d} w}{1-\rho_K^*}  = \dfrac{w}{w_{bd}}\overset{\eqref{eqn:assump_2b}}{<} 1. \label{eqn:r_lim}
\end{align}

Since $\lim_{t \rightarrow \infty} R(t) < 1$ and $0< R(t) < R(t-1) \, \forall t$, from Claim~\ref{thm:clm2} there exists $T' < \infty$ such that $R(t) < 1 \, \forall t > T'$.  
Then, we have
\begin{align}
    & \Pi_{k=0}^t R(k) = \Pi_{k=0}^{T'} R(k) \, \Pi_{k=T'+1}^t R(k) < \Pi_{k=0}^{T'} R(0) \, \Pi_{k=T'+1}^t R(T'+1) < \left(R(0)\right)^{T'+1} \, \left(R(T'+1)\right)^{t-T'} \nonumber \\
    \implies & \lim_{t \rightarrow \infty} \Pi_{k=0}^t R(k) = 0, \label{eqn:x3}
\end{align}
since $R(T'+1) < 1$ and $R(0)$ is constant.

Now we bound the second term on the right hand side of~\eqref{eqn:x2}. For $t > T'$ we have,
\begin{align*}
   & R(0)...R(t) + R(1)...R(t) + ... + R(T')R(T'+1)...R(t) + R(T'+1)...R(t) + ... R(t-1)R(t) + R(t) + 1 \\
   < & \left(R(0)...R(T')\right) \, \left(R(T'+1)\right)^{t-T'} + \left(R(1)...R(T')\right) \, \left(R(T'+1)\right)^{t-T'} + ... + R(T')\left(R(T'+1)\right)^{t-T'} + \\
   & \left(R(T'+1)\right)^{t-T'} + ... + \left(R(T'+1)\right)^{2} + R(T'+1) + 1 \\
   = & \underbrace{\left(\left(R(0)...R(T')\right) + ... + R(T') \right)}_{constant} \left(R(T'+1)\right)^{t-T'}  + 1 + R(T'+1) + \left(R(T'+1)\right)^{2} + ... + \left(R(T'+1)\right)^{t-T'}.
\end{align*}
Since $R(T'+1) < 1$, we have
\begin{align}
    \lim_{t \rightarrow \infty} \left(R(t) + R(t) R(t-1) + ... + R(t)...R(0) \right) < \dfrac{1}{1 - R(T'+1)}. \label{eqn:x4}
\end{align}
The first statement follows from~\eqref{eqn:x2},~\eqref{eqn:x3} and~\eqref{eqn:x4}. The second statement follows by taking limit and using~\eqref{eqn:r_lim}.
